# Supplementary material for: SCPL: Enhancing Neural Network Training Throughput with Decoupled Local Losses and Model Parallelism
Source: arXiv:2602.00062 source file (2026-02-03)
Supplement: Supplementary file 1 [file appendix.tex]

\section{Appendix} \label{sec:app}

\subsection{Details of experimental settings} \label{app:detailed-settings}

In our vision tasks, both BP and SCPL adopt a cosine learning rate scheduler, starting from an initial learning rate of 10e-3 and decaying to 10e-5. We use Adam as the optimizer. For data augmentation, we refer to the settings in~\citep{khosla2020supervised} on CIFAR-10 and CIFAR-100, where each image undergoes resizing, random cropping, random horizontal flipping, jittering, and random grayscaling to generate two augmented views as inputs. Consequently, the batch size increases from the original $N$ to $2N$. Regarding the batch size in training time measurement experiments, both are tested under 32, 64, 128, 256, and 512. For the accuracy comparison, the batch size of BP is set to 128 and SCPL is set to 1024. However, as shown in Figure~\ref{fig:lstm-agnews-bs-vs-acc}, Figure~\ref{fig:lstm-imdb-bs-vs-acc}, Figure~\ref{fig:transformer-agnews-bs-vs-acc}, and Figure~\ref{fig:transformer-imdb-bs-vs-acc}, SCPL mostly performs better than or comparable to BP for various batch sizes. The training epochs are set to 200. In the SCPL configuration, all models use an MLP (multi-layer perceptron) as the projection head, with a structure of $Linear(dim, 512)-ReLU()-Linear(512, 1024)$. Here, $dim$ represents the dimension after flattening the feature map. The temperature parameter $\tau$ is set to 0.1 for all models. Furthermore, each component is placed on a separate GPU in the training time experiments. The detailed configurations for VGG and ResNet are as follows.

\begin{itemize}
\item VGG consists of 4 max-pooling layers (MP) and 6 convolutional layers (Conv). Each convolutional layer uses ReLU as the activation function and employs batch normalization (BN). The classifier consists of 2 fully connected layers (FC) with a sigmoid as the activation function. In our implementation, SCPL splits VGG into 4 components, structured as ${component}_1 - {component}_2 - {component}_3 - {component}_4$. The ${component}_1$ and ${component}_2$ are composed of $[[Conv - BN - ReLU] \times 2 - MP]$. The ${component}_3$ and ${component}_4$ are composed of $[[Conv - BN - ReLU] - MP]$. However, an additional classifier is included in ${component}_4$, resulting in $[{component}_4 - [FC - sigmoid - FC]]$.
\item ResNet is an 18-layer residual neural network (ResNet-18) with a linear, fully connected layer as the classifier. In our implementation, SCPL splits ResNet into 4 components, structured as ${component}_1 - {component}_2 - {component}_3 - {component}_4$. The ${component}_1$ is structured as $[StemBlock - BasicBlock \times 2]$. The ${component}_2$, ${component}_3$, and ${component}_4$ are structured as $[BasicBlock \times 2]$. However, an additional classifier is included in the last ${component}_4$, resulting in $[{component}_4 - [FC]]$. The $StemBlock$ includes $[Conv - BN - ReLU]$. The $StemBlock$ comprises a convolutional layer followed by batch normalization (BN) and Rectified Linear Unit (ReLU) activation. The $BasicBlock$ is constructed with a convolutional layer using the LeakyReLU activation function, another convolutional layer, and a skip connection that adds a fully connected transformation to the input of the $BasicBlock$ module. Finally, the output passes through another LeakyReLU activation.
\end{itemize}

Both BP and SCPL use a fixed learning rate of $10e-3$ in NLP tasks and employ Adam as the optimizer. All texts in the datasets undergo preprocessing steps of creating word indices, removing stop words, and limiting the maximum text word length $T$, a hyperparameter representing each sample's sentence length. Data augmentation is not utilized; therefore, the batch size remains at its original value $N$. The maximum text word length per sample for the AG's news dataset is set to 60, while for IMDB, it is set to 350. The training epochs for both BP and SCPL models are set to 50. Regarding the batch size, we experimented with 16, 32, 64, 128, 256, 384, 512, 768, 1024, 1280, 1536, 1792, 2048, and 4096, and we present the results with the best accuracy in this paper. Additionally, both BP and SCPL models utilize pre-trained Glove word embeddings~\citep{pennington2014glove} of dimensionality 300 in the first layer of the model. In the configuration of SCPL, all models, by default, use an identity function, $f(x) = x$, as the projection head. The temperature parameter $\tau$ is set to 0.1 for all models.

Detailed architectures of LSTM and Transformer are as follows.

\begin{itemize}
\item LSTM consists of 3 bi-LSTM hidden layers (each with a dimensionality of 300) and 1 Glove embedding layer at the beginning of the model. At the end of the model, 2 fully connected layers serve as the classifier. The Tanh function is used as the activation function between the two layers. SCPL splits the LSTM model into 4 components, structured as ${component}_1 - {component}_2 - {component}_3 - {component}_4$. ${Component}_1$ represents the $[GloveEmb]$ layer, while ${component}_2$, ${component}_3$, and ${component}_4$ represent the $[LSTM]$ layers. However, an additional classifier is included in ${component}_4$, resulting in $[{component}_4 - [FC-tanh-FC]]$.

\item The Transformer consists of 3 Transformer encoders (each with a dimensionality of 300 and a dropout rate of 0.1) and 1 Glove embedding layer at the beginning of the model. At the end of the model, 2 fully connected layers serve as the classifier. The Tanh function is used as the activation function between the two layers. SCPL splits the Transformer model into 4 components, structured as ${component}_1 - {component}_2 - {component}_3 - {component}_4$. ${Component}_1$ represents the $[GloveEmb]$ layer, while ${component}_2$, ${component}_3$, and ${component}_4$ represent the $[Transformer]$ layers. However, an additional classifier is included in ${component}_4$, resulting in $[{component}_4 - [FC-tanh-FC]]$.
\end{itemize}
